# Supplementary material for: Ultrafast terahertz-field-driven ionic response in ferroelectric BaTiO$_3$
Source: arXiv:1608.08470 source file (2016-10-31)
Supplement: Supplementary file 1 [file supplementalmaterials_final.pdf]

# Supplemental Materials of "Ultrafast terahertz-field-driven ionic response in ferroelectric $BaTiO_3$"

## 1. Sample preparation and characterization.

90 nm thick BTO thin-films were grown epitaxially on $NdScO_3$ $(110)_O$ single-crystal substrates (Crystec, GmbH) using established procedures. Briefly, the films were deposited via pulsed-laser deposition using a KrF excimer laser (LPX 305, Coherent). The films were grown in 20 mTorr of oxygen at 600 °C from a BTO ceramic target at a laser repetition rate of 2 Hz and a laser fluence of 1.4 J/cm$^2$ in an on axis-geometry. Prior to growth, the target was sanded, cleaned, and sufficiently preablated to assure that the target surface had reached steady state. Following growth, the films were cooled to room temperature at 5°C/min. in a 760 Torr oxygen pressure. The X-ray diffraction characterization of the sample is shown in Fig. S1 and the the AFM and PFM characterization of the sample is shown in Fig. S2.

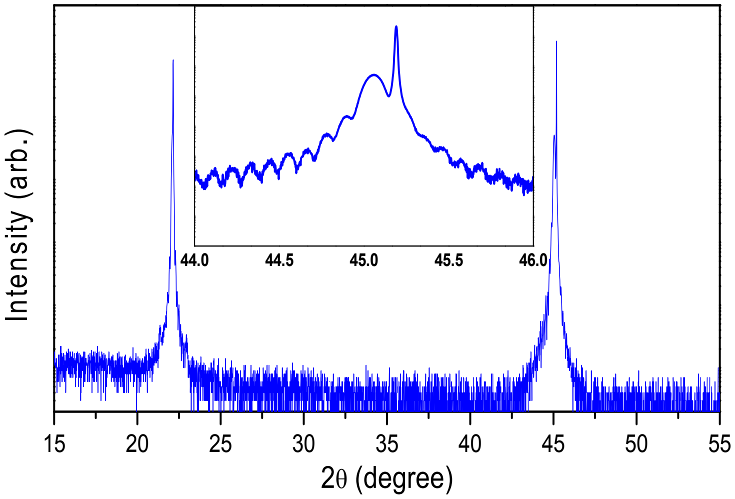


Fig. S1. θ-2θ scan of BTO/NSO reflections showing almost lattice matched thin film peak at slightly lower angles relative to the NSO substrate reflection. Spacing between fringes is consistent with estimated film thickness (90 nm).

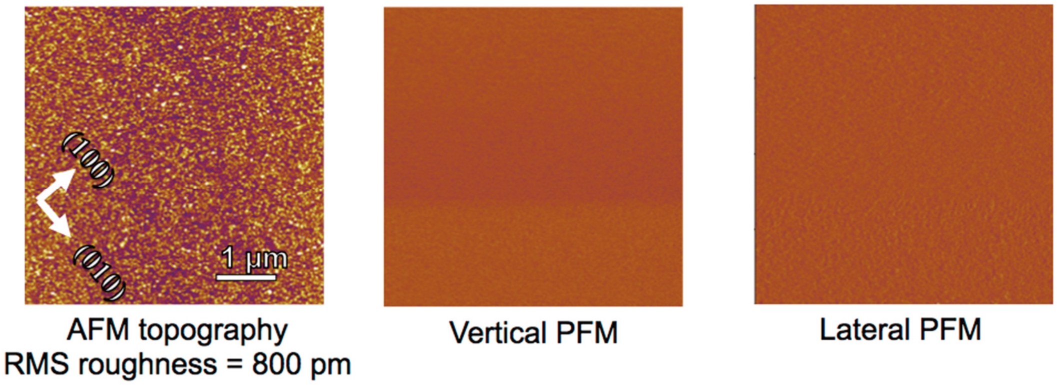


Fig. S2. Piezo-force microscopy and AFM images of the BTO thin film.

## 2. Temperature-dependent x-ray diffraction measurements.

Temperature-dependent x-ray diffraction (XRD) measurements are used to quantify the temperature change induced by the THz-field excitation. However, there is a significant difference between the THz pump and temperature-dependent XRD measurements: During the THz excitation only the film is heated while the substrate remains at room temperature whereas in a static heating measurement both substrate and film are heated. Since the film is epitaxially clamped to the substrate, this leads to significantly different responses: We show in the following that the out-of-plane lattice of the $BaTiO_3$ (BTO) film expands as a result of THz-induced ionic heating, in contrast to the lattice contraction observed on heating using a heating stage. In particular, we describe below a quantitative extraction of effective thermal expansion coefficients under THz excitation, which can then be used to quantify the mechanisms by which the THz field drives long-lived changes in the c-axis lattice constant.

Temperature-dependent measurements were conducted using Cu-$K\alpha$ radiation on the (002) BTO reflection and allow us to estimate the heating induced by the THz pump. The measured temperature dependent x-ray diffraction curves are shown in Fig. S3, showing shifts of both the film and substrate peaks, with the substrate peaks shifting to lower 2θ and the film peak shifting to higher 2θ with increasing temperature. The measured strain of the film with increasing temperature is shown in Fig. S4.

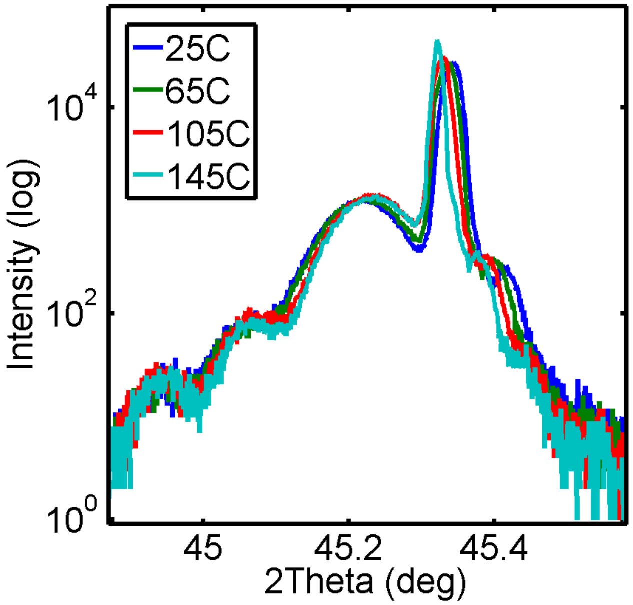


Fig. S3. Temperature-dependent x-ray diffraction curves for the (002) reflection showing both the film and substrate reflections.

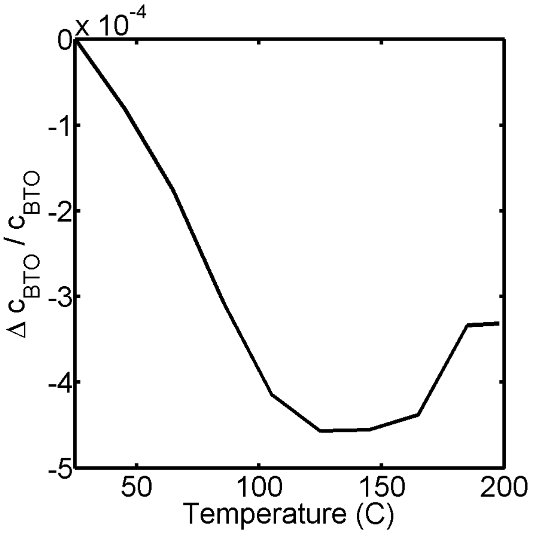


Fig. S4. Temperature-dependent relative strain measured from the (002) reflection of the BTO thin film peak.

Here we account for the clamping effect and correct for it to obtain the intrinsic out-of-plane response of the BTO film. For a transversely isotropic film like BTO,

$$\begin{pmatrix} \epsilon_x \\ \epsilon_y \\ \epsilon_z \end{pmatrix} = \begin{pmatrix} S_{11} & S_{12} & S_{13} \\ S_{12} & S_{11} & S_{13} \\ S_{13} & S_{13} & S_{33} \end{pmatrix} \begin{pmatrix} \sigma_x \\ \sigma_y \\ \sigma_z \end{pmatrix} + \begin{pmatrix} \alpha_a \\ \alpha_a \\ \alpha_c \end{pmatrix} \Delta T$$

where $S$ is the elastic compliance matrix with four independent elements. For the case of an isotropic thin film with $\varepsilon_x = \varepsilon_y$, $\sigma_x = \sigma_y$, and $\sigma_z=0$ (corresponding to a free surface), one finds that

$$\epsilon_x = (S_{11} + S_{12})\sigma_x + \alpha_a \Delta T$$

$$\epsilon_z = 2S_{13}\sigma_x + \alpha_c \Delta T$$

Solving for $\varepsilon_z$ one obtains:

$$\epsilon_z = \frac{2S_{13}}{S_{11} + S_{12}}(\epsilon_x - \alpha_a \Delta T) + \alpha_c \Delta T$$

This equation encodes how an in-plane strain (for example a mismatch strain between the film and substrate) leads to an out-of-plane strain. It also includes the ordinary contribution determined by the thermal expansion coefficient $\alpha_c$. If the film is clamped to the substrate then $\varepsilon_x=\alpha_s \Delta T$ and we find

$$\epsilon_z = \frac{2S_{13}}{S_{11} + S_{12}}(\alpha_s - \alpha_a)\Delta T + \alpha_c \Delta T$$

As an example, for the case where in-plane expansion of the substrate dominates over the film, the first term is typically negative (since $S_{13} < 0$) and this effect will act in the same direction as the typically negative thermal expansion coefficient along the c-axis, associated with a reduction in tetragonality near the Curie temperature. This effect is shown in Fig. S3 with the BTO peak shifting to higher angle with

increasing temperature. In the temperature dependent experiment, we directly measure $\varepsilon_z$ as a function of temperature through:

$$\epsilon_z = -\cot(\theta_B)\Delta\theta(T)$$

where $\Delta\theta(T)$ is the temperature-dependent shift of the Bragg peak and $\theta_B$ is the Bragg angle. Using experimentally determined values for the in-plane thermal expansion coefficient of the $NdScO_3$ (NSO) substrate (~3.65 x $10^{-6}$ $K^{-1}$) and literature values for the in-plane expansion coefficient of BTO (~6 x $10^{-6}$ $K^{-1}$)[1], one can then extract from the experimental data above an effective c-axis thermal expansion coefficient for the BTO film by solving the above equations. Near room temperature, one obtains a value for $\alpha^c_{BTO}$ ~ -4 x $10^{-6}$ $K^{-1}$ with the negative value reflecting the reduction of the tetragonality as the film is heated towards the Curie temperature.

When we excite the thin film with short-pulse THz fields and drive a temperature jump, there is no time for the in-plane strain to change on the short time-scales of the experiment. There is, however, an in-plane stress that builds up which impacts the out-of-plane strain. One can understand this in a general sense using the thermoelastic relation

$$\sigma_i = C_{ij}(\varepsilon_j - \alpha_j \Delta T)$$

where the $C_{ij}$'s are the elastic constants, related to the $S_{ij}$'s above through well-known relations and $\alpha_j=(\alpha_a, \alpha_a, \alpha_c)^T$ encodes the anisotropic thermal expansion coefficients. Here we neglect shear effects. For transversely isotropic symmetry, one finds using the above equation that the time-dependent stress in the out-of-plane direction satisfies

$$\sigma_z = C_{33}\epsilon_z - (2C_{13}\alpha_a + C_{33}\alpha_C)\Delta T$$

where we have taken the in-plane strain values to be zero by the argument above. The second term in this equation represents the externally induced thermoelastic stress or pressure which reduces to the known result[2]

$$\sigma_{ext} = -3B\alpha\Delta T$$

for the case of an isotropic medium where B is the bulk modulus. It has a dependence on both time and space with

$$\Delta T(z,t) = \begin{cases} \Delta T, & t > 0; 0 < z < L \\ 0, & otherwise \end{cases}$$

where $L$ is the thickness of the film. This assumes homogeneous energy deposition by the THz field, justified by the known optical constants at 1 THz.

The equation for the stress together with the equation of motion,

$$\rho\frac{\partial^2 u}{\partial t^2} = \frac{\partial \sigma_z}{\partial z}$$

leads to a wave equation describing the coherent acoustic phonon response of the film, e.g.

$$C_{33}\frac{\partial^2 \epsilon_z}{\partial z^2} - \frac{\partial^2 P}{\partial z^2} = \rho\frac{\partial^2 \epsilon_z}{\partial t^2}$$

where in this case

$$P = (2C_{13}\alpha_a + C_{33}\alpha_c)\Delta T(z,t)$$

is the induced homogeneous stress within the film and ρ is the density. For the case of BTO, using known values for the elastic constants and with $\alpha_a$ positive and $\alpha_c$ negative, the quantity P is positive for increases in the temperature of the sample, reflecting a temperature-induced tensile stress in the film, as experimentally observed.

The time-dependent solution of the above differential equations is associated with tensile strains starting at both the top free interface and at the buried interface[3] and traveling at the acoustic velocity into the film in counter-propagating directions, with the amplitude of the ingoing wave given by

$$\epsilon_z = \frac{P}{C_{33}} = \frac{1}{C_{33}}(2C_{13}\alpha_a + C_{33}\alpha_c)\Delta T$$

This is also the long time strain after the acoustic waves have propagated fully through the film, corresponding to an effective thermal expansion coefficient

$$\alpha_{eff} = \frac{2C_{13}\alpha_a + C_{33}\alpha_c}{C_{33}}$$

Using the expansion coefficients value we calculated previously and using literature values of the thermoelastic coefficients of $C_{13}$ = 114 GPa and $C_{33}$ = 160 GPa [4], we determined an effective expansion coefficient of ~5 x $10^{-6}$ $K^{-1}$. The strain driven by the THz at the highest fields inside the split ring resonator (SRR) structure within the film of 0.7 MV/cm was 3.6 x $10^{-4}$ which then corresponds to a temperature *increase* of ~72K, in reasonable agreement with the estimated temperature rise in Section 3. Taking the calculated time-dependent strains as solutions of the wave equation above and using these as an input to a dynamical diffraction model for the scattering of x-rays from inhomogeneous strains, we can quantitatively fit the observed time-dependent changes as shown in Fig. 2(b,c,d) to this model, including also a transient structure factor modulation as discussed above.

### **3. Structure factor calculations**.

To estimate the unit cell rearrangements that can give rise to an increase in the diffracted intensity at the (003) peak of ~1% as observed, we calculate the structure factor change as a function of the displacement of the central Ti atom. The initial structure factor at time zero can be approximated as the following, neglecting contribution from the oxygen atoms

$$F_{003} = f_{Ba} - f_{Ti}\exp(-6\pi i\delta)$$

where it is assumed that the initial polarization state is associated with an out-of-plane displacement δ of the Ti atom from the center of the unit cell, measured with respect to the lattice parameter (~4 Å). The negative contribution from the Ti atom shows, as noted in the main text, that this scattering contribution is out-of-phase with respect to that of the Ba atom. For small displacements, the scattered x-ray intensity is then

$$I_0 \sim |F_{003}|^2 \sim (f_{Ba} - f_{Ti})^2 + 36 f_{Ba} f_{Ti}\pi^2\delta^2$$

If the THz pulse induces an out-of-plane vibrational excitation of the Ti atom with amplitude A(t), the time-dependent structure factor is then

$$F(t) \sim f_{Ba} - f_{Ti}\exp[-6\pi i(\delta + A(t))]$$

For an incoherent response after averaging over many unit cells, we assume $\langle A(t)\rangle \sim 0$ and $\langle A^2(t)\rangle = A^2_{RMS}(t)$, which is justified by the MD simulation shown in Section 8, the time-dependent scattered x-ray intensity is then:

$$I(t) \sim |F(t)|^2 \sim (f_{Ba} - f_{Ti})^2 + 36 f_{Ba} f_{Ti} \pi^2 (\delta^2 + A^2_{RMS}(t))$$

$$I(t) \sim I_0 + 36 f_{Ba} f_{Ti} \pi^2 A^2_{RMS}(t)$$

This gives an approximate expression for the change in diffracted intensity as a function of the amplitude A

$$\frac{\Delta I}{I_0} \sim \frac{36 f_{Ba} f_{Ti} \pi^2 A^2_{RMS}(t)}{(f_{Ba} - f_{Ti})^2}$$

This shows that induced incoherent displacements give rise to an increase in the scattering efficiency for the (003) reflection, corresponding to a reduction in the destructive interference between the Ba and Ti atoms, as observed. Using tabulated values for the scattering factors, this corresponds to an induced RMS displacement of the Ti atom of 0.03 Å for a 1% modulation, comparable to the static displacement of the Ti atom associated with the intrinsic ferroelectric polarization[5] and consistent with the estimates from the MD simulations (see Methods).

*Measurements on BTO (012) reflection.* We also carried out measurements probing the THz-driven response on the (012) asymmetric reflection of BTO, probing on the high angle side of the reflection (Fig. S5). This reflection has sensitivity to the in-plane response of the film, along the direction perpendicular to the applied THz field and the ferroelectric polarization. For this reflection, under the approximation that the in-plane Ti motion perpendicular to the applied THz field is not excited (as also predicted by simulations, see section 8 of the supplementary, Fig. S12c), one expects that the time-dependent structure factor can be written as:

$$F(t) \sim f_{Ba} + f_{Ti}\exp\left[-2\pi i\left(1\left(\frac{1}{2}\right) + 2\left(\frac{1}{2} + \delta + A(t)\right)\right)\right] = f_{Ba} - f_{Ti}\exp[-4\pi i(\delta + A(t))]$$

and thus should be modulated $6^2/4^2=2.25\times$ smaller than that for the (003) reflection. Accounting as well for the differences in the scattering factors, this gives an estimate of ~3× smaller diffraction intensity change compared to the (003) peak, well within the noise of the measurements shown below. In contrast, the long-lived response, associated with THz-driven heating is clearly resolved.

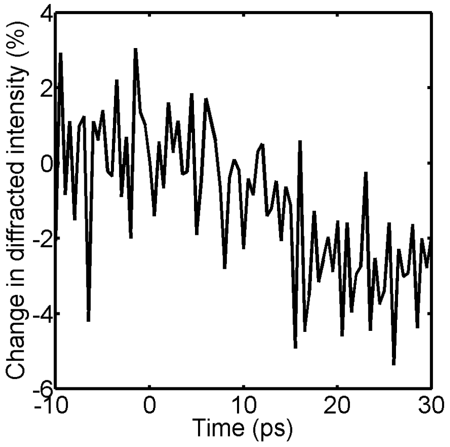


Fig. S5. THz-pump / x-ray probe measurements on (012) BTO reflection

**4. Measurements of the optical properties of the BTO/NSO film and THz heating estimates.**

Previous studies have investigated the optical properties of $BaTiO_3$ in both thin film and bulk form at terahertz frequencies[6,7], all showing significant absorption associated with low frequency/soft modes overlapping with the spectrum of the applied THz pulse. We carried out additional measurements to confirm this, particularly since the optical properties for BTO on NSO substrates have not been previously reported to our knowledge. Using an oscillator-driven photoconductive switch THz emitter with bandwidth up to ~3 THz, we measured the transmitted THz waveforms using electro-optic sampling through both a BTO/NSO sample and a pure NSO substrate. Figure S4a shows the measured time-domain waveforms comparing the signal without sample to the two samples (Air, NSO and BTO/NSO) (Blue, Gray, and Black lines respectively). The waveform with sample is delayed, mainly associated with the refractive index of the 500 μm substrate from which we extract an index of refraction of the substrate of ~4.8, consistent with prior far infrared measurements in other rare-earth scandates [8]. We note that the substrate thicknesses were almost but not exactly equal, such that some of the observed delay in the BTO/NSO vs. pure NSO is associated with this thickness difference (in addition to reflecting the large dielectric constant of the BTO). However, it is also clear that the transmitted beam for the BTO/NSO sample is significantly reduced compared to that of the pure substrate. Fig. S6b shows the transmission amplitudes in the frequency domain and Fig. S6c shows the extracted frequency-dependent index of refraction of the substrate. For the case considered here, where the THz field is applied transversely to the ferroelectric polarization, previous studies indicate large transverse susceptibilities [9], and we see evidence for this here. A detailed analysis and extraction of the frequency-dependent n and k for the BTO film is beyond the scope of this paper, but it is clear from the data shown that there is significant interaction of the THz field with the film, with this effect turning on at a frequency of about 0.5 THz, well within the applied THz spectrum for the experiments considered in the main text. The spectrum of the THz pulse used for the THz pump measurements is shown in Fig.S5.

The observed reduction in transmission then enables one to calculate an approximate temperature jump. Because of the uncertainties discussed above, we present two separate calculations in the following: From the above discussion, convolving the observed frequency dependent response with the THz spectrum (shown in Fig. S7), let us approximate this as ~10% of the incident light is absorbed. For an applied incident THz fluence ~100 $\mu J/cm^2$and taking into account an estimated ~10% absorption and a 10× field enhancement for the SRR metamaterial, this gives a peak absorbed fluence $F_A$ ~1 mJ/cm.[2] This then

corresponds to a temperature jump of ~ $F_A/(C\rho L)$ ~ 40K (where C is the specific heat = 0.4 J/gK, ρ is the density = 6 g/cc, and L is the film thickness = 90 nm). Alternatively, taking measured values for n and k for BTO thin films from Misra et al. [6] one can estimate an effective THz conductivity from the relation $\sigma=2\varepsilon_0\omega nk$ from which one obtains $\sigma\sim 40\ (\Omega cm)^{-1}$ (note this includes vibrational contributions and is many orders of magnitude larger than the DC conductivity). In the thin film limit, the electric field within the film is simply determined by the optical properties of the substrate[10,11] e.g. $E_{inside}=2E_{app}/(n_s+1)$ from which one estimates a peak field of 700 kV/cm within the film using the measured value for the index of refraction of the NSO substrate. Using these values, one may estimate the temperature jump from the deposited energy density $\sigma E^2\tau$, where τ is the THz pulse duration (1/0.5 THz ~ 2 ps), to be ~ 20K, in good agreement with the estimate above. These estimates are also in good agreement with the temperature at long times estimated from our experimentally measured shifts in the Bragg peak position.

We also note that, from the estimated temperature jumps observed, one can estimate whether THz-driven electronic responses (e.g. tunneling ionization, impact ionization etc.) are responsible for the observed effects. For the experimentally measured ΔT=72 K temperature jump, this corresponds to an energy density U in the film of U= $\Delta T\rho C$ ~ 100 J/cc. For carriers excited to energies of order 0.1 eV above the conduction band edge by nonlinear field-drive processes, this would then require a carrier density of ~$10^{22}$/cc for heating through electron-phonon coupling. This is many orders of magnitude larger than, for example, the induced carrier density in GaAs at similar field strengths (1 MV/cm), of order $10^{17}$/cc [12].

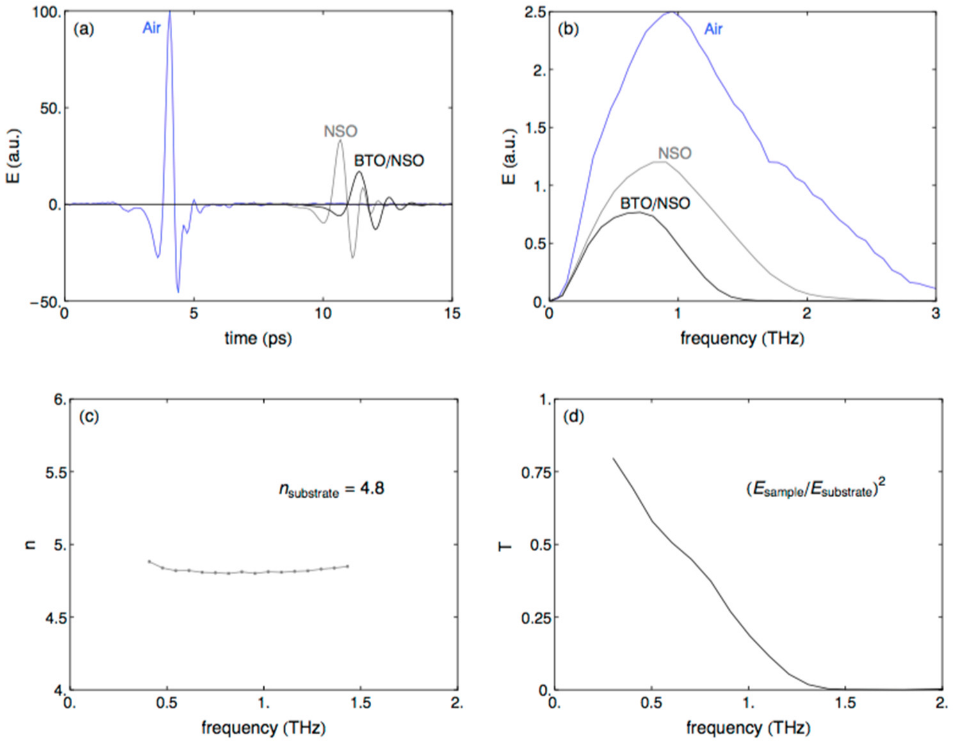


Fig. S6. THz spectroscopic measurements of sample in transmission using a broader band photoconductive switch THz emitter. a) Raw waveforms for air, substrate and sample + substrate respectively. b) Frequency-resolved transmission for three samples. c) Extracted frequency-dependent index of refraction of NSO substrate. d) Frequency-dependent transmission $(E_{sample}/E_{substrate})^2$.

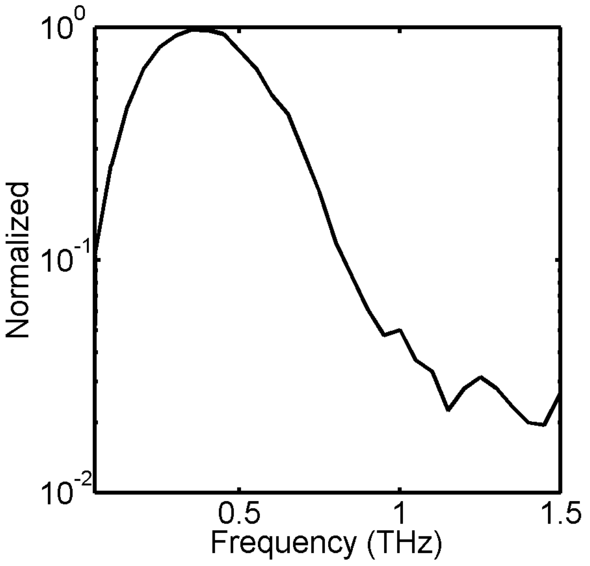


Fig. S7. Spectrum of applied THz pulse obtained by Fourier transform of measured THz waveform shown in main text.

**5. Simulation of film temperature as a function of time**

The cooling of the film is a result of thermal transport from the film to the substrate. We model the system as a heterostructure consisting of a 90 nm $BaTiO_3$ (BTO) film and 0.5 mm NSO substrate. To simplify the calculation, we assume there is no phase transition involved. Following a similar treatment in the supplementary materials of Ref. [13], the thermal transport can be described by a one-dimensional thermal diffusion equation:

$$\frac{dT(t,z)}{dt} = \left(\frac{\kappa}{C_p\rho}\right)\frac{d^2T(t,z)}{dz^2},$$

with boundary conditions:

$$C_p\rho\frac{dT(t,z)}{dt} = -g\frac{dT(t,z)}{dz}|_{z=D} \text{and } \frac{dT(t,z)}{dz}|_{z=0} = 0$$

where $T$ is the temperature profile as functions of time delay *t* and depth *z*. To avoid the complication from across ferroelectric to paraelectric phase transition, we simulate the thermal transport at a base temperature of 470 K. Following the THz excitation, the film temperature is elevated from the base temperature of 470 K to $T(0 < z < D, t = 100\,ps) = 542$ K. The average film temperature at any instant in time can be obtained by $T(t) = \frac{1}{D}\int_0^D T(t,z)dz$. Using thermal parameters of the BTO thin film and NSO substrate in Table 1, the thermal diffusion equation is numerically solved to obtain the film temperature $T$ as a function of time delay shown in Fig.3b in the main text.

| | |
|---|---|
| BTO film thickness $D$ | 90 nm |
| BTO Density ρ | 6.02 g/cm$^3$ |
| NSO Density ρ | 6.11 g/cm$^3$ |
| Thermal conductivity (BTO) $\kappa_1$ [14] | 4.8 W/(m·K) at 300 K<br>4.1 W/(m·K) at 470 K |
| Thermal conductivity (NSO) $\kappa_2$ (approximated from measured values for $NdGaO_3$)[15] | 8 W/(m·K) |
| Kaptiza (interfacial) conductance $g$ (no prior measured value, quoted as the best fit parameter to the measured response) | 10000 W/(K·cm$^2$) |
| Specific heat (BTO) $C_{1p}$ [14] | 103 J/(mol·K) at 300 K<br>114 J/(mol·K) at 470 K |
| Specific heat (NSO) $C_{2p}$ [16] | 127 J/(mol·K) |

Table 1. Thermal parameters of the sample.

**6. Field dependence at higher fields.**

Measurements within electrode structures investigated the field dependence of the response up to peak incident fields of 2 MV/cm (see also section 6 following). Fig. S8 shows the change in the diffracted intensity at t=200 ps as a function of the applied field (with field enhancement), measured at the half-rising point on the lower angle side of the (002) rocking curve peak. This shows a response consistent with the quadratic response observed on shorter time scales.

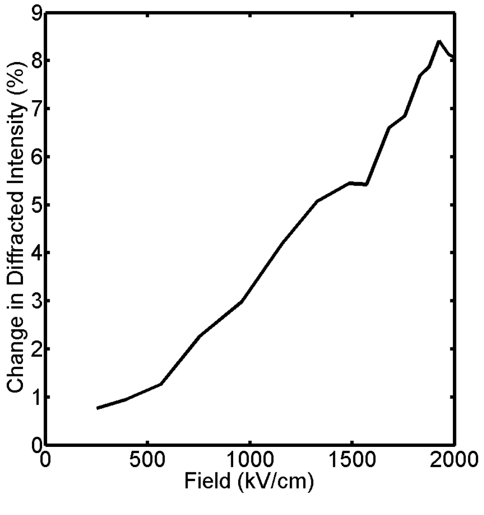


Fig. S8. Quadratic field dependence of the change in diffracted intensity as a function of SRR-enhanced applied THz field

## 7. Field Enhancement Simulations.

3D simulations were run using CST-Microwave Studio on the metamaterial structures using the frequency domain solver at 1 THz and applying periodic boundary conditions on the SRR unit cell shown below in Fig. S9. The incident THz peak field of 200 kV/cm is enhanced by the SRR to 2 MV/cm within the gap in vacuum. For a thin film, we expect the THz field inside the film to be reduced by a factor of $2/(n+1)$, where $n$ is the index of refraction of the substrate. Using the value for $n$ measured above, the peak field within the thin film is estimated to be ~700 kV/cm.

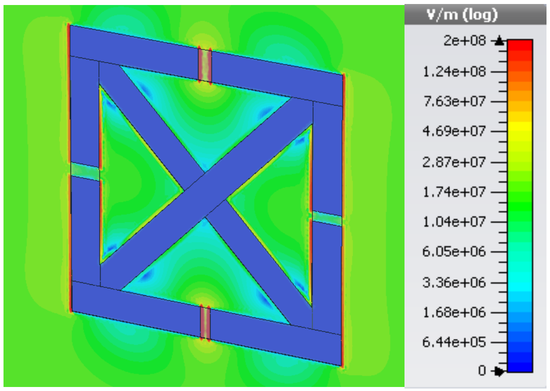


Fig. S9. FDTD simulations for the split-ring resonator devices.

## 8. The experimental setup

The THz pump, x-ray diffraction probe measurements on ps time scales were conducted at the Linac Coherent Light Source (LCLS) at the SLAC National Accelerator Laboratory [17]. Single-cycle THz pulses were generated using a tilted-pulse front technique to provide an electric field bias on sub-ps time-scales, applied such that the field within the sample is orthogonal to the ferroelectric polarization (Fig. 1). The symmetric (003) and (002) reflections were mainly used as a probe of the THz-driven structural changes. Additional data on the (012) reflection is included as well. Measurements at the LCLS utilized 50 femtosecond x-ray pulses at 7 keV and 120 Hz repetition rate as a probe, recording the diffracted x-ray beam in a specular geometry on a pixel array detector and reading out each shot on a pulse-by-pulse basis, with peak applied fields of 600 kV/cm. Pump and probe beams were synchronized to each other with a timing jitter of approximately 200 fs.

The THz pump, x-ray diffraction probe measurements on ns time scales were conducted at the 7-ID-C beamline of the Advanced Photon Source (APS). The broadband THz pulses with peak electric fields up to 200 kV/cm at the sample position is generated by an ultrafast Ti:Sapphire laser system that provides 60 fs, 800 nm, 2 mJ laser pulses at 1 kHz repetition rate. Gold split-ring resonators are used to further enhanced the THz field. The square-shaped unit structure is $50\times50$ μm$^2$ and the gap size is 2.7 μm shown in Fig. S10. The polarization of the THz fields are aligned along the vertical edges of the SRR structure. Monochromatic hard x-ray pulses with 11 keV photon energy and 100 ps pulse duration were focused by a Fresnel zone plate to a spot size of 450 nm (full width of half maximum along the vertical direction). X-rays diffracted from the (002) Bragg peak of the BTO thin film were measured at APS (in contrast to the (003) reflection probed at LCLS) by a gated x-ray area detector. The time delay between x-ray and THz pulses could be electronically controlled and the time resolution is set by the 100 ps x-ray pulse duration. The sample temperature was controllable by a heating stage from 300 K to 500 K.

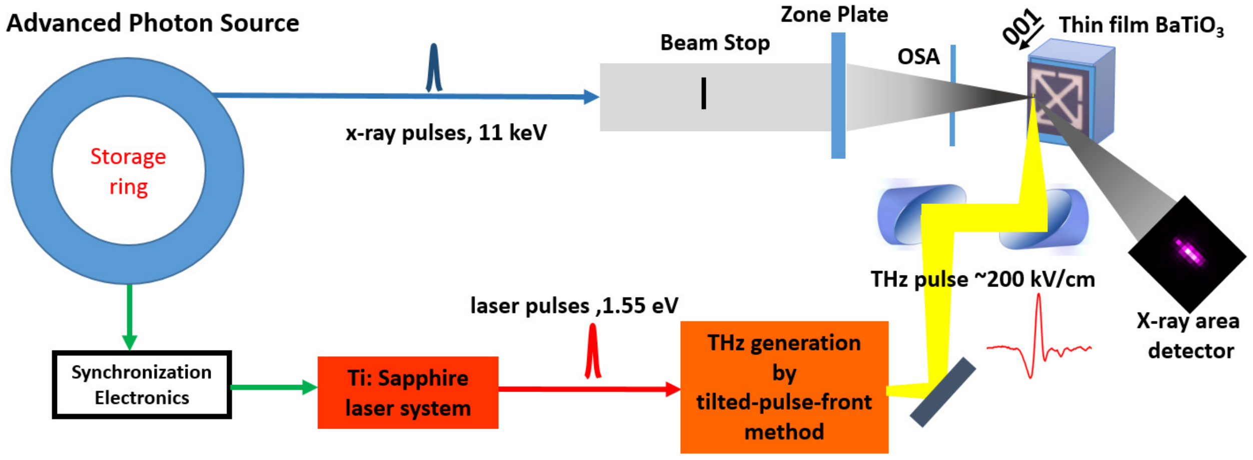


Fig. S10. The experimental setup of the THz pump/hard x-ray microdiffraction probe experiments at the Advanced Photon Source.

## 9. Molecular Dynamics (MD) simulations

Molecular dynamics simulations of bulk BTO are conducted with a 10$\times$10$\times$10 perovskite-type supercell containing 5000 atoms using a bond-valence-based interatomic potential. The pressure is maintained at 0.1 MPa by the Parrinello-Rahman barostat and the temperature is controlled by the Nosé–Hoover thermostat implemented in LAMMPS [20]. The bond-valence-based interatomic potential is parameterized from density functional theory calculations and can reproduce temperature-driven phase transitions of BTO accurately. A single cycle THz pulse is applied along [010] direction, which is perpendicular to the direction of the polarization along [001] direction. To model the clamping effect of the substrate, the supercell dimensions along [100] and [010] directions are fixed. The instantaneous local polarization, $\mathbf{P}_u(t)$, for each unit cell is calculated with

$$\boldsymbol{P_u}(t) = \frac{1}{V_u}\left(\frac{1}{8}\boldsymbol{Z}_{Ba}^{*}\sum_{i=1}^{8}\boldsymbol{r}_{Ba,i}(t) + \boldsymbol{Z}_{Ti}^{*}\boldsymbol{r}_{Ti}(t) + \frac{1}{2}\boldsymbol{Z}_{O}^{*}\sum_{i=1}^{6}\boldsymbol{r}_{O,i}(t)\right),$$

where $V_u$ is the volume of a unit cell, $\boldsymbol{Z}_{Ba}^{*}$, $\boldsymbol{Z}_{Ti}^{*}$, and $\boldsymbol{Z}_{O}^{*}$ are the Born effective charges of Ba, Ti, and O atoms. $\boldsymbol{r}_{Ba,i}(t)$, $\boldsymbol{r}_{Ti,i}(t)$, and $\boldsymbol{r}_{O,i}(t)$ are instantaneous atomic positions of Ba, Ti, and O atoms in a unit cell obtained from MD simulations. The instantaneous total polarization of the supercell is the average value of $\mathbf{P}_u(t)$. To capture the stochastic behavior of electric-field-driven ferroelectric response, we perform 20 simulations starting from different equilibrium structures, and the average over the obtained 20 trajectories is used to evaluate the structural and dynamical properties (shown in Figure 4). It is noted that the nearly-periodic high-frequency oscillation of the polarization (Figure 4f) is an artifact due to the usage of thermostat/barostat to control temperature/pressure. The frequency of the oscillation that reflects the heat transfer speed between the system and the thermostat is closely related to the value of the effective mass of thermostat/barostat (defined as damping parameters in LAMMPS). We find that the time scale of the polarization decay after the THz field also depends on the damping parameters. Despite the intrinsic imperfectness (periodic fluctuation of temperature and pressure) of the Nosé-Hoover thermostat and Parrinello-Rahman barostat, the suppression of the out-of-plane polarization is found to be universal, regardless of the values of damping parameters.

The simulation volume consisted of 10×10×10 unit cells and a total of 20 different runs were performed with slightly modified initial configurations. The motions of the Ti atoms were extracted relative

to each unit cell by fixing the Ba atom as the origin, and the collective Ti displacements were averaged for each run. The final plots include the average of the 20 runs. Shown in Fig. S11a is the THz excitation pulse and the corresponding in-plane motion of the Ti atom (Fig. S11b). The RMS out-of-plane motion of the Ti atom as shown in the main text is calculated as $\sqrt{\langle\delta^2\rangle - \langle\delta\rangle^2}$, where $\delta$ is the displacement of the Ti atom from its equilibrium position. The structure factor was similarly calculated neglecting contribution from oxygen atoms for each unit cell and averaged over the 1000 unit cells. The modulus squared of the structure factor is proportional to the x-ray scattering intensity. Fig. S12 shows analogous simulations of the time-dependent polarization modulation along (a) $P_z$ (out-of-plane, parallel to ferroelectric polarization), (b) $P_x$ (in-plane, parallel to the applied THz field), (c) $P_y$ (in-plane, perpendicular to the applied THz field), (d) and of the total polarization. This shows as expected that the dominant response is an adiabatic response along the direction of the applied THz field, with negligible response in the in-plane perpendicular direction, all consistent with a rotation effect. Fig. S12e shows the magnitude of the time-dependent polarization rotation, consistent with those expected based on the large transverse susceptibility of BTO [9].

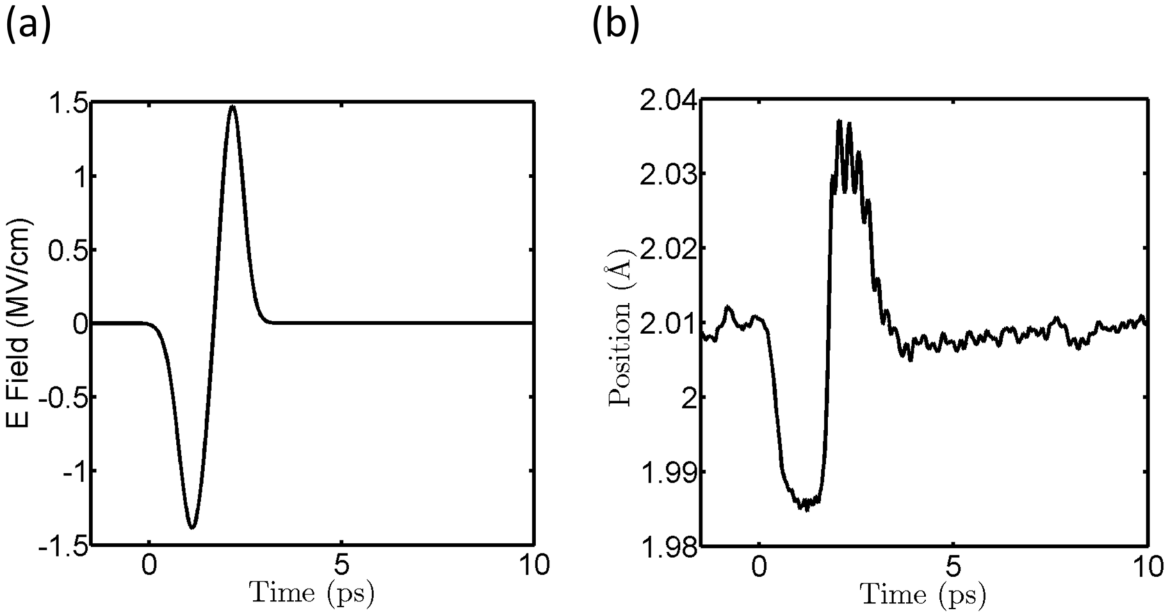


Fig. S11. (a) Excitation THz electric field profile used in MD simulation. (b) Ti atom position in the in-plane direction parallel to the THz field.

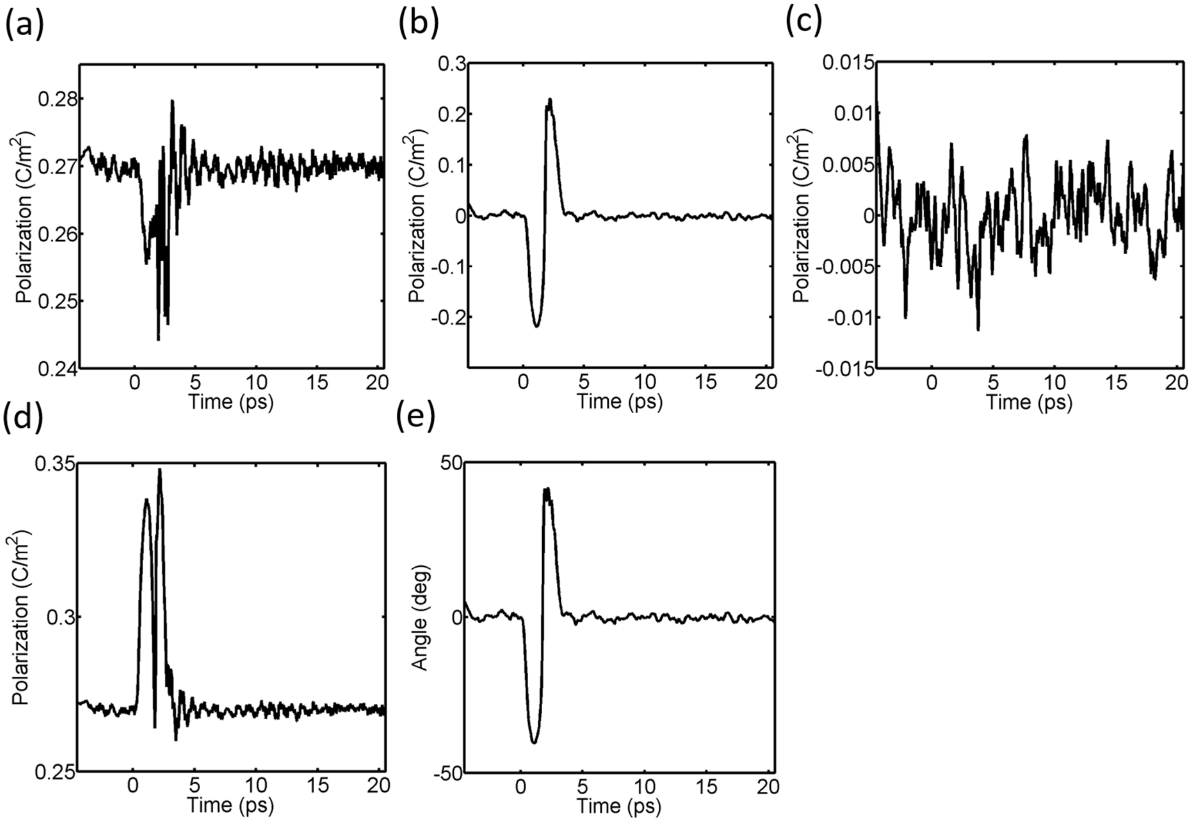


Fig. S12. Simulations of the time-dependent polarization modulation of (a) $P_z$ (out-of-plane, parallel to ferroelectric polarization), (b) $P_x$ (in-plane, parallel to the applied THz field), (c) $P_y$ (in-plane, perpendicular to the applied THz field), (d) and of the total polarization. (e) Calculated polarization rotation angle as a function of time.

REFERENCES

[1] Y. He, Thermochimica Acta **419**, 135 (2004).
[2] C. Thomsen, H. T. Grahn, H. J. Maris, and J. Tauc, Physical Review B **34**, 4129 (1986).
[3] M. Nicoul, U. Shymanovich, A. Tarasevitch, D. von der Linde, and K. Sokolowski-Tinten, Appl. Phys. Lett. **98**, 191902 (2011).
[4] Z. Li, S. K. Chan, M. H. Grimsditch, and E. S. Zouboulis, J. Appl. Phys. **70**, 7327 (1991).
[5] M. B. Smith, K. Page, T. Siegrist, P. L. Redmond, E. C. Walter, R. Seshadri, L. E. Brus, and M. L. Steigerwald, Journal of the American Chemical Society **130**, 6955 (2008).
[6] M. Misra, K. Kotani, T. Kiwa, I. Kawayama, H. Murakami, and M. Tonouchi, Applied Surface Science **237**, 421 (2004).
[7] T. Hoshina, K. Kanehara, H. Takeda, and T. Tsurumi, Jpn. J. Appl. Phys. **53**, 09PD03 (2014).
[8] L. Baldassarre, A. Perucchi, S. Lupi, and P. Dore, J. Phys. Condens. Matter **22**, 355402 (2010).
[9] M. Davis, M. Budimir, D. Damjanovic, and N. Setter, J. Appl. Phys. **101**, 054112 (2007).
[10] F. Chen, J. Goodfellow, S. Liu, I. Grinberg, M. C. Hoffmann, A. R. Damodaran, Y. Zhu, P. Zalden, X. Zhang, I. Takeuchi, A. M. Rappe, L. W. Martin, H. Wen, and A. M. Lindenberg, Adv. Mater. **27**, 6371 (2015).

[11] T. F. Heinz, *Second-Order Nonlinear Optical Effects at Surfaces and Interfaces* (Elsevier, 1991).

[12] H. Hirori, K. Shinokita, M. Shirai, S. Tani, Y. Kadoya, and K. Tanaka, Nature Communications **2**, 594 (2011).

[13] H. Wen, P. Chen, M. P. Cosgriff, D. A. Walko, J. H. Lee, C. Adamo, R. D. Schaller, J. F. Ihlefeld, E. M. Dufresne, D. G. Schlom, P. Evans, J. Freeland, and Y. Li, Phys. Rev. Lett. **110**, 037601 (2013).

[14] S. T. Davitadze, S. N. Kravchun, B. A. Strukov, B. M. Goltzman, V. V. Lemanov, and S. G. Shulman, Appl. Phys. Lett. **80**, 1631 (2002).

[15] W. Schnelle, R. Fischer, and E. Gmelin, Journal of Physics D: Appl. Phys. **34**, 846 (2001).

[16] R. Uecker, D. Klimm, R. Bertram, M. Bernhagen, I. Schulze-Jonack, M. Brützam, A. Kwasniewski, T. M. Gesing, and D. G. Schlom, Acta. Physica Polonica A **124**, 295 (2013).

[17] M. Chollet, R. Alonso-Mori, M. Cammarata, D. Damiani, J. Defever, J. T. Delor, Y. Feng, J. M. Glownia, J. B. Langton, S. Nelson, K. Ramsey, A. Robert, M. Sikorski, S. Song, D. Stefanescu, V. Srinivasan, D. Zhu, H. T. Lemke, and D. M. Fritz, The X-ray Pump-Probe instrument at the Linac Coherent Light Source, J. Synchrotron Rad. **22**, 503 (2015).

[18] M. Seo and H. Park, Nat. Photon. **3**, 152 (2009).

[19] M. Liu, H. Y. Hwang, H. Tao, A. C. Strikwerda, K. Fan, G. R. Keiser, A. J. Sternbach, K. G. West, S. Kittiwatanakul, J. Lu, S. A. Wolf, F. G. Omenetto, X. Zhang, K. A. Nelson, and R. D. Averitt, Nature **487**, 345 (2012).

[20] S. Plimpton, Journal of Computational Physics **117**, 1 (1995).
